# Supplementary material for: An unlikely route to low lattice thermal conductivity: small atoms in a simple layered structure
Source: arXiv:1804.01517 source file (2018-04-04)
Supplement: Supplementary file 1 [file mg3sb2-supplemental.pdf]

# Supplemental information

April 3, 2018

## 1 Experimental equations and table

Due to the lack of experimental speed of sound data in most of the compounds, we used the calculated bulk and shear elastic moduli from Materials Project to estimate $\nu_s$ [1]. For an isotropic material, a specific C11 and C44 value at each temperature can be obtained by fitting the peak positions of the spectrum, from which C12, poisson ratio P, Young's modulus Y , shear modulus G, longitudinal and transverse speed of sound $v_l$ and $v_t$ are given by:

$$C_{12} = C_{11} - 2C_{44}; P = \frac{C_{12}}{C_{11}+C_{12}}; \; Y = 2(P+1)C_{44}; \; G = C_{44}; \; B = \frac{YC_{44}}{2C_{44}+3Y}; \; v_L = \sqrt{\frac{B+\frac{4}{3}G}{\rho}}; \; v_T = \sqrt{\frac{G}{\rho}}.$$

Table 1: Density, predicted and experimental elastic moduli and speed of sound at room temp for all of the $A\text{Mg}_2Pn_2$ samples. The calculated CTE is extracted from the phonon dispersion by relaxing the position of the atoms and shape of the unit cell at different fixed volumes in the framework of the quasiharmonic approximation at 300K. The calculated Young's, shear and bulk modulus is from Materialsproject.org. Unit cell volume is from ICSD data base and the density is calculated from Molar mass and unit cell volume.

| | $Mg_3Sb_2$ | | $CaMg_2Sb_2$ | | $CaMg_2Bi_2$ | | $YbMg_2Bi_2$ | | $YbMg_2Sb_2$ | | $Mg_3Bi_2$ | |
|---|---|---|---|---|---|---|---|---|---|---|---|---|
| | Exp | Cal | Exp | Cal | Exp | Cal | Exp | Cal | Exp | Cal | Exp | Cal |
| Young's modulus (GPa) | 41.13 | 50 | 69.62 | 64 | 58.82 | 54 | 57.99 | - | 72.05 | 68 | 35.98 | 39 |
| Shear modulus (GPa) | 15.68 | 19 | 28.25 | 26 | 23.71 | 22 | 23.34 | - | 29.35 | 28 | 13.39 | 15 |
| Bulk modulus (GPa) | 36.41 | 42 | 43.35 | 39 | 37.77 | 35 | 37.51 | - | 44 | 41 | 38.39 | 37 |
| $v_L$ ($ms^{-1}$) | 3794 | 4094 | 4562 | 3138 | 3538 | 3438 | 3137 | 2988 | 3888 | 3783 | 3120 | 3123 |
| $v_T$ ($ms^{-1}$) | 1984 | 2138 | 2694 | 2010 | 2068 | 2010 | 1829 | 1705 | 2310 | 2262 | 1522 | 1602 |
| Avg speed of sound ($ms^{-1}$) | 2587 | 2790 | 3317 | 3207 | 2558 | 2486 | 2265 | 2133 | 2836 | 2769 | 2055 | 2109 |
| Volume CTE ($10^{-5}K^{-1}$) | 5.19 | 6.27 | - | 4.62 | 4.44 | 5.06 | 4.56 | - | - | - | 6.09 | - |
| Density ($gcm^{-3}$) | 4.041 | | 3.871 | | 5.656 | | 7.160 | | 5.473 | | 5.843 | |
| Unit cell volume ($A^3$) | 130.081 | | 142.551 | | 148.804 | | 148.388 | | 141.191 | | 139.544 | |
| Molar mass ($gmol^{-1}$) | 316.435 | | 332.208 | | 506.6488 | | 639.6248 | | 465.184 | | 490.8758 | |
| $1/B * \partial B/\partial T$ ($10^{-4}K^{-1}$) | -3.6 | - | - | - | -1.69 | - | -1.51 | - | - | - | -2.78 | - |

## 2 Phonon band structures and Grüneisen parameters

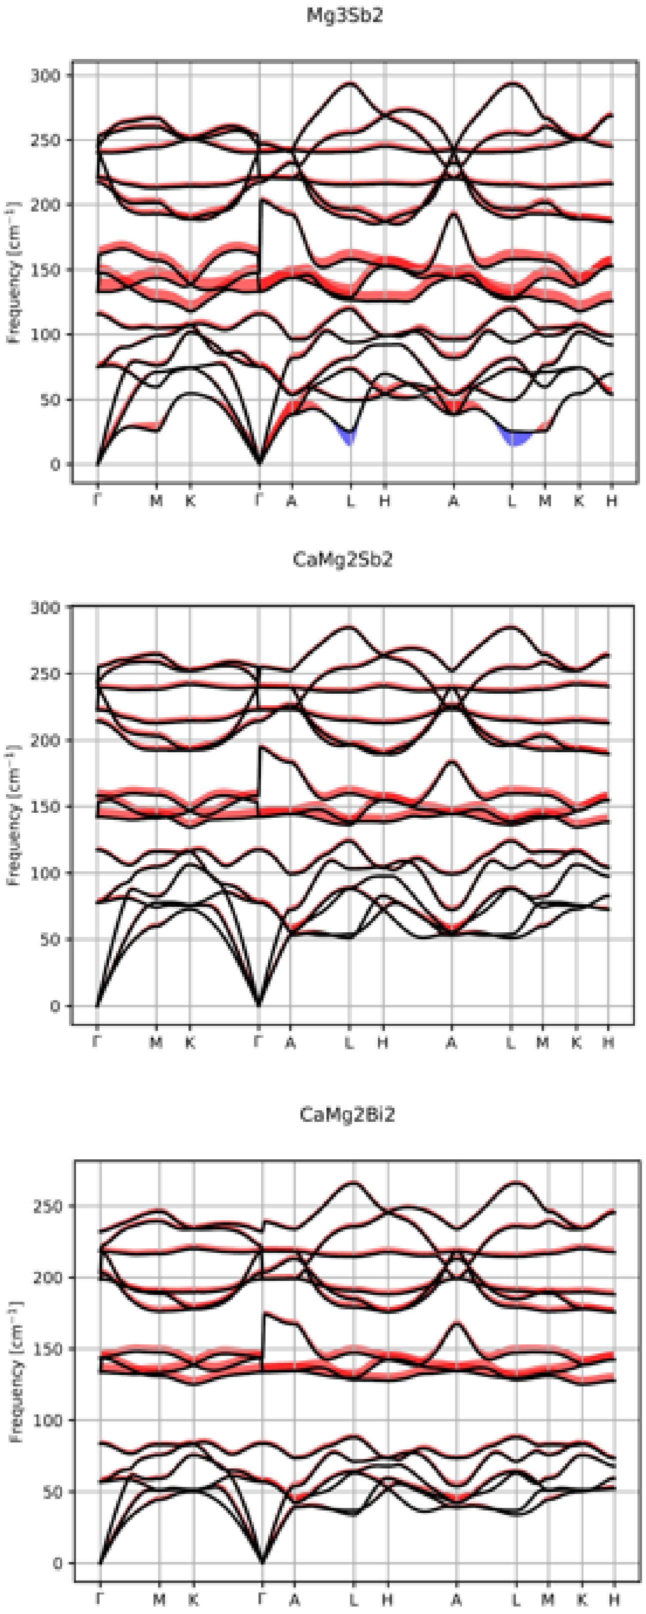


Figure 1: Phonon band structure with Grüneisen parameters for $Mg_3Sb_2$, $CaMg_2Sb_2$ and $CaMg_2Bi_2$. The colored areas represent the values of the Grüneisen parameters.

From the values of $\gamma_{i,q}$, where $i$ labels the modes and $q$ the q-points in the Brillouin zone, it is possible to extract an average value for the Grüneisen parameters. Several possible definitions are present in literature to calculate that, see e.g. Refs.[2] and [3]. Here we use the definition given in Eq. (7) of Ref.[4] (also Eq (6) in Ref.[2]) that averages the square of the Grüneisen parameters weighted with the contribution of each modes to the heat capacity $C_i, q$, evaluated at the Debye temperature $\theta_{\mathrm{D}}$:

$$\gamma = \sqrt{\overline{\gamma}^2} = \sqrt{\frac{\sum_i \sum_q \gamma_{i,q}^2 C_{i,q}}{\sum_i \sum_q C_{i,q}}} \tag{1}$$

$$\theta_{\mathrm{D}} = n^{-1/3} \sqrt{\frac{5\hbar}{3k_b^2} \frac{\int_0^\infty \omega^2 g(\omega) d\omega}{\int_0^\infty \omega^2 g(\omega) d\omega}}, \tag{2}$$

where $g(\omega)$ is the phonon DOS as a function of the frequency $\omega$ and $n$ is the number of atoms in the cell. where $g(\omega)$ is the phonon DOS as a function of the frequency $\omega$ and $n$ is the number of atoms in the cell.

One can then use the values of $\gamma$ to estimate the lattice thermal conductivity $\kappa_l$ according to the Slack model (see Eq.(1) of Ref.[2] or Eq.(4) of Ref.[3].

Table 2: Values of the average Grüneisen parameters and lattice thermal conductivity as obtained from the models described in the text. According to the analysis reported in literature, these models often tend to overestimate the value of the thermal conductivity. Nonetheless they confirm the lower $\kappa_l$ of $Mg_3Sb_2$ compared to the other two materials.

| | $Mg_3Sb_2$ | $CaMg_2Sb_2$ | $CaMg_2Bi_2$ |
|---|---|---|---|
| $\gamma$ | 1.83 | 1.44 | 1.46 |
| $\kappa_l$ | 9.42 | 17.58 | 21.56 |

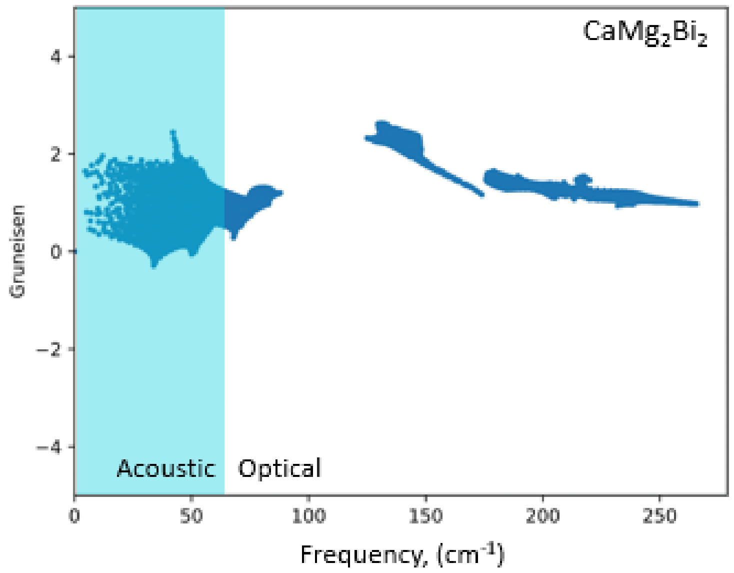


Figure 2: The mode Grüneisen parameters as a function of frequency for $CaMg_2Bi_2$ is similar to $CaMg_2Sb_2$.

# 3 Computed temperature-dependent elastic moduli and thermal expansion

Given the knowledge of $V(T)$, where $V$ is the volume of the system, we can evaluate the evolution of the elastic constants as a function of $T$. This requires the calculation of the elastic constants at different volumes. In Fig.3 we report the variation of the Young's modulus $Y$ with respect to the value at 300 K as a function of $T$. $Mg_3Sb_2$ displays a greater variation of $Y$ compared to $CaMg_2Sb_2$ and $CaMg_2Bi_2$.

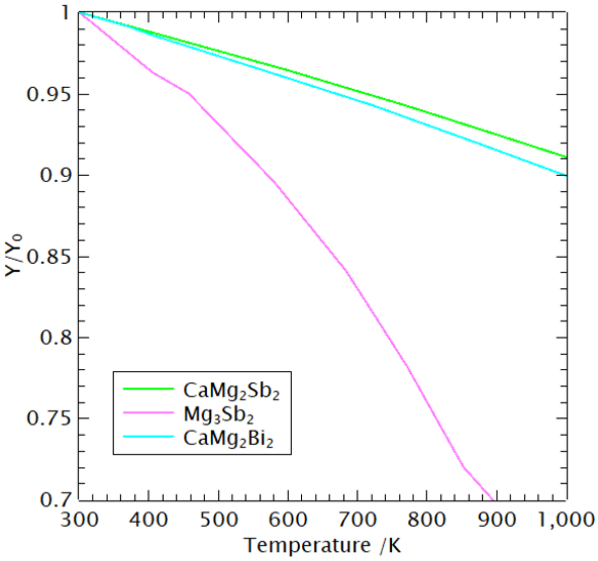


Figure 3: The computed temperature-dependent elastic moduli of $Mg_3Sb_2$, $CaMg_2Sb_2$, and $CaMg_2Bi_2$.

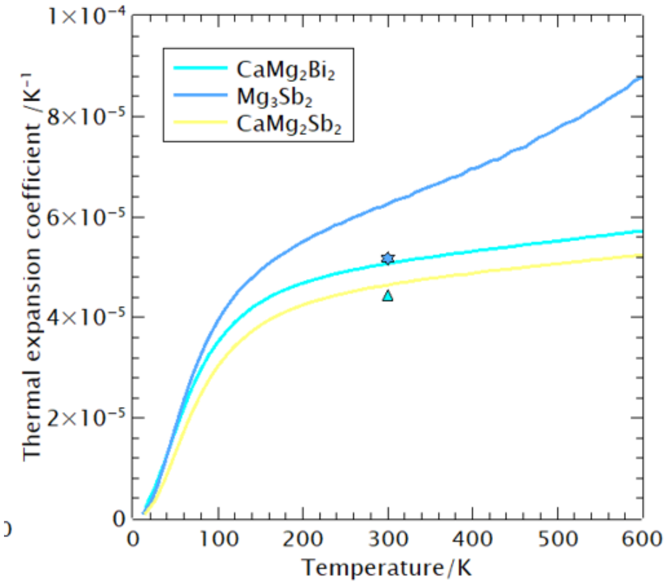


Figure 4: The computed thermal expansion of $Mg_3Sb_2$, $CaMg_2Sb_2$, and $CaMg_2Bi_2$.

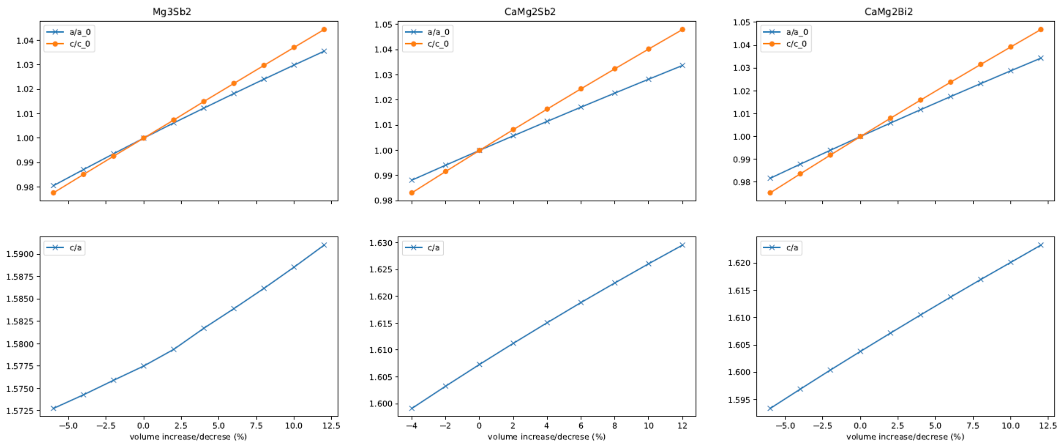


Figure 5: Differences in lattice expansion in the $xy$ plane and along the $z$ axis.

# 4 Frozen phonons

In order to further highlight the anharmonicity of the modes at the edge of the Brillouin zone of $Mg_3Sb_2$, we have performed frozen phonon calculation. The calculation consists in displacing the atoms along following the eigen-displacements of a specific phonon mode and calculate the total energy of the new configuration. The procedure is repeated for different amplitudes of the displacements (always with the same directions). In Fig. 6 we report the values of the energies obtained from self-consistent DFT calculations at various displacements (dots) and the energies expected in the case the system was completely harmonic (solid lines). The last quantity si calculated using the phonon frequency as a coefficient for the quadratic term of the expression $E = E_0 + ad^2$, where $d$ is the amplitude of the displacement.

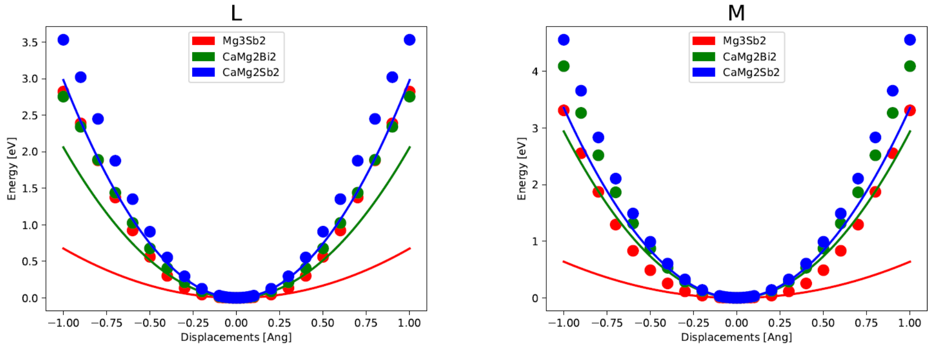


Figure 6: Comparison between the values of the energies obtained from self-consistent DFT calculations at various displacements (dots) and the energies expected in the case the system was completely harmonic (solid lines) for eigendisplacements of the lower acoustic mode at the $L$ (left) and $M$ (right) point of the Brillouin zone.

# 5 Born effective charges

The Born effective charges (BECs) $Z^*$ are included in the phonon calculations to obtain the correct LO-TO splitting. Their value can give information about the polarizability of the material. The

value of the BECs for each element of the material in the $xy$ plane and along the $z$ axis are reported in Table 3.

For all the sites the BECs are quite close among the different materials. $Mg_3Sb_2$ shows a larger value of $Z^*$ for the first atom of $A_1M_2X_2$ compound, compared to $CaMg_2Sb_2$ and $CaMg_2Bi_2$. This suggests a more covalent bond between the first Mg and Sb compared to the bond between Ca and Sb/Bi. This seems to be confirmed by the ELF as well.

Table 3: Values of the Born effective charges in the $xy$ plane and along the $z$ axis. Atoms of the same line are corresponding between the three materials.

| $Mg_3Sb_2$ | | | $CaMg_2Bi_2$ | | | $CaMg_2Sb_2$ | | |
|---|---|---|---|---|---|---|---|---|
| | $Z^*_{xy}$ | $Z^*_z$ | | $Z^*_{xy}$ | $Z^*_z$ | | $Z^*_{xy}$ | $Z^*_z$ |
| Mg | 3.21 | 3.06 | Ca | 2.58 | 2.67 | Ca | 2.46 | 2.57 |
| Mg | 1.86 | 1.85 | Mg | 1.84 | 1.76 | Mg | 1.82 | 1.77 |
| Sb | -3.47 | -3.38 | Bi | -3.13 | -3.10 | Sb | -3.05 | -3.06 |

# References


[1] M. De Jong, W. Chen, T. Angsten, A. Jain, R. Notestine, A. Gamst, M. Sluiter, C. K. Ande, S. Van Der Zwaag, J. J. Plata, *et al.*, "Charting the complete elastic properties of inorganic crystalline compounds," *Sci. Data*, vol. 2, p. 150009, 2015.

[2] P. Nath, J. J. Plata, D. Usanmaz, C. Toher, M. Fornari, M. B. Nardelli, and S. Curtarolo, "High throughput combinatorial method for fast and robust prediction of lattice thermal conductivity," *Scripta Materialia*, vol. 129, pp. 88–93, 2017.

[3] L. Bjerg, B. B. Iversen, and G. K. Madsen, "Modeling the thermal conductivities of the zinc antimonides znsb and zn 4 sb 3," *Physical Review B*, vol. 89, no. 2, p. 024304, 2014.

[4] G. K. Madsen, A. Katre, and C. Bera, "Calculating the thermal conductivity of the silicon clathrates using the quasi-harmonic approximation," *physica status solidi (a)*, vol. 213, no. 3, pp. 802–807, 2016.
